# Supplementary material for: A First Step Towards Detecting Values-violating Defects in Android APIs
Source: arXiv:2109.14359 source file (2021-09-29)
Supplement: Supplementary file 1 [file Appendix.tex]

\begin{appendices}

\section{API detection rule implementation}
\label{appendix:detectors}

This appendix contains the implementation of the algorithms in section III
\begin{algorithm}
\label{algorithm:Animation hedonism}
	\caption{Animation hedonism violation detector}
	\begin{flushleft}
        \textbf{INPUT:} : $JavaPath$ java file path\\
        \textbf{OUTPUT:} return a boolean value: \\
            \qquad $True$: violation exist \\
            \qquad $False$: violation does not exist
    \end{flushleft}
	\begin{algorithmic}[1]
	    \State /*using deep first search to search all the AST nodes out*/
	    \State $AstNodes \leftarrow $ search( $JavaPath$ )
		\State $ViolationList\leftarrow $ an empty list
		\State $VarNames\leftarrow $ an empty list
		\For {\textbf{all} $AstNode$ $in$ $AstNodes$}
		\If{$AstNode$ $is$ Variable Decelerator Node}
		\If{"Animator" in $AstNode$.name}
		\State append $AstNode$.name \textbf{to} $VarNames$
		\EndIf
		\EndIf
		\If{$AstNode$ $is$ Method Invocation Node $and$ $AstNode$.qualifier $in$ $VarNames$}
		
		\If{$AstNode$.member = \textbf{"setDuration"}}
		\For{$argument$ $in$ $AstNode$.arguements}
		\If{$argument$.member \textgreater 2000}
		\State append \textbf{"Violation"}\textbf{to} $ViolationList$
		\EndIf
		\EndFor
		\EndIf
		
		\If{$AstNode$.member = \textbf{"setRepeatCount"}}
		\For{$argument$ $in$ $AstNode$.arguements}
		\If{$argument$.member = "Infinity"}
		\State append \textbf{"Violation"} $in$ $ViolationList$
		\EndIf
		\EndFor
		
		\EndIf
		\EndIf
		
		\EndFor
		\For{ \textbf{all} $ListElement$ $in$ $ViolationList$}
		\If{$ListElement$ = \textbf{"Violation"}}
		\State \textbf{Return} True
		\EndIf
		\EndFor
		\State \textbf{Return} False
		
	\end{algorithmic} 
\end{algorithm}

\begin{algorithm}
\label{algorithm:Hardware security}
	\caption{Hardware security violation detector}
	\begin{flushleft}
        \textbf{INPUT:} : $JavaPath$ java file path\\
        \textbf{OUTPUT:} return a boolean value: \\
            \qquad $True$: violation exist \\
            \qquad $False$: violation does not exist
    \end{flushleft}
	\begin{algorithmic}[1]
	    \State /*using deep first search to search all the AST nodes out*/
	    \State $AstNodes \leftarrow $ search( $JavaPath$ )
		\State $ViolationList\leftarrow $ an empty list
		\State $VarNames\leftarrow $ an empty list
		\For {\textbf{all} $AstNode$ $in$ $AstNodes$}
		\If{$AstNode$ $is$ Variable Decelerator Node}
		\If{\textbf{"Camera"} = $AstNode$.name \textbf{and} \textbf{"CameraDevice"} = $AstNode$.name}
		\State append $AstNode$.name \textbf{to} $VarNames$
		\EndIf
		\EndIf
		\If{$AstNode$ $is$ Method Invocation Node $and$ $AstNode$.qualifier $in$ $VarNames$}
		
		\If{$AstNode$.member = \textbf{"takePicture"} or $AstNode$.member = \textbf{"createCaptureSession"}}
		\State append \textbf{"Violation"} $in$ $ViolationList$
		
		\EndIf
		\EndIf
		
		\EndFor
		\For{ \textbf{all} $ListElement$ $in$ $ViolationList$}
		\If{$ListElement$ = \textbf{"Violation"}}
		\State \textbf{Return} True
		\EndIf
		\EndFor
		\State \textbf{Return} False
		
	\end{algorithmic} 
\end{algorithm}

\begin{algorithm}
\label{algorithm:Mtp self direction violation}
	\caption{Mtp self direction violation detector}
	\begin{flushleft}
        \textbf{INPUT:} : $JavaPath$ java file path\\
        \textbf{OUTPUT:} return a boolean value: \\
            \qquad $True$: violation exist \\
            \qquad $False$: violation does not exist
    \end{flushleft}
	\begin{algorithmic}[1]
	    \State /*using deep first search to search all the AST nodes out*/
	    \State $AstNodes \leftarrow $ search( $JavaPath$ )
	    \State /*names of methods which we want to collect about data transmission*/
		\State $MethodIdentifyList\leftarrow $ an empty list
	    \State /*names of methods which we collected in java file*/
		\State $MethodList\leftarrow $ an empty list
		\State $VarNames\leftarrow $ an empty list
		\For {\textbf{all} $AstNode$ $in$ $AstNodes$}
		\If{$AstNode$ $is$ Variable Decelerator Node}
		\If{\textbf{"MtpDevice"} = $AstNode$.name}
		\State append $AstNode$.name \textbf{to} $VarNames$
		\EndIf
		\EndIf
		\If{$AstNode$.member $in$ $MethodIdentifyList$ $and$ $AstNode$.qualifier $in$ $VarNames$}
		
		\State append $AstNode$.member $to$ $MethodList$
		
		\EndIf
		
		\EndFor
		\If{$MethodList$ have data transmission function with only one direction}
		\State \textbf{Return} True
		\EndIf
		\State \textbf{Return} False
		
	\end{algorithmic} 
\end{algorithm}

\begin{algorithm}
\label{algorithm:Media self direction and hedonism}
	\caption{Media self direction and hedonism detector}
	\begin{flushleft}
        \textbf{INPUT:} : $JavaPath$ java file path\\
        \textbf{OUTPUT:} return a boolean value: \\
            \qquad $True$: violation exist \\
            \qquad $False$: violation does not exist
    \end{flushleft}
	\begin{algorithmic}[1]
	    \State /*using deep first search to search all the AST nodes out*/
	    \State $AstNodes \leftarrow $ search( $JavaPath$ )
	    \State /*names of methods which we want to collect about media playing and stop*/
		\State $MethodIdentifyList\leftarrow $ an empty list
	    \State /*names of methods categorized by different object which we collected in java file*/
		\State $MethodDict\leftarrow $ an empty dictionary
		\State $VarNames\leftarrow $ an empty list
		\For {\textbf{all} $AstNode$ $in$ $AstNodes$}
		\If{$AstNode$ $is$ Variable Decelerator Node}
		\If{\textbf{"MediaPlayer"} = $AstNode$.name}
		\State append $AstNode$.name \textbf{to} $VarNames$
		\EndIf
		\EndIf
		\If{$AstNode$.member $in$ $MethodIdentifyList$ $and$ $AstNode$.qualifier $in$ $VarNames$}
		
		\State append $AstNode$.member $to$ $MethodDict[AstNode.member]$
		
		\EndIf
		
		\EndFor
		\If{$MethodDict$ have media play functions but not stop functions for all MediaPlayer object}
		\State \textbf{Return} True
		\EndIf
		\State \textbf{Return} False
		
	\end{algorithmic} 
\end{algorithm}

\begin{algorithm}
\label{algorithm:Telephony conformity and security}
	\caption{Telephony conformity and security violation detector}
	\begin{flushleft}
        \textbf{INPUT:} : $JavaPath$ java file path\\
        \textbf{OUTPUT:} return a boolean value: \\
            \qquad $True$: violation exist \\
            \qquad $False$: violation does not exist
    \end{flushleft}
	\begin{algorithmic}[1]
	    \State /*using deep first search to search all the AST nodes out*/
	    \State $AstNodes \leftarrow $ search( $JavaPath$ )
		\State $ViolationList\leftarrow $ an empty list
		\State $VarNames\leftarrow $ an empty list
		\For {\textbf{all} $AstNode$ $in$ $AstNodes$}
		\If{$AstNode$ $is$ Variable Decelerator Node}
		\If{\textbf{"SmsManager"} = $AstNode$.name}
		\State append $AstNode$.name \textbf{to} $VarNames$
		\EndIf
		\EndIf
		\If{$AstNode$ $is$ Method Invocation Node $and$ $AstNode$.qualifier $in$ $VarNames$}
		
		\If{$AstNode$.member is message sending function name}
		\State append \textbf{"Violation"} $in$ $ViolationList$
		
		\EndIf
		\EndIf
		
		\EndFor
		\For{ \textbf{all} $ListElement$ $in$ $ViolationList$}
		\If{$ListElement$ = \textbf{"Violation"}}
		\State \textbf{Return} True
		\EndIf
		\EndFor
		\State \textbf{Return} False
		
	\end{algorithmic} 
\end{algorithm}

\begin{algorithm}
\label{algorithm:Nfc security}
	\caption{Nfc security violation detector}
	\begin{flushleft}
        \textbf{INPUT:} : $JavaPath$ java file path\\
        \textbf{OUTPUT:} return a boolean value: \\
            \qquad $True$: violation exist \\
            \qquad $False$: violation does not exist
    \end{flushleft}
	\begin{algorithmic}[1]
	    \State /*using deep first search to search all the AST nodes out*/
	    \State $AstNodes \leftarrow $ search( $JavaPath$ )
		\State $MethodInovationList\leftarrow $ an empty list
		\State $VarNames\leftarrow $ an empty list
		\For {\textbf{all} $AstNode$ $in$ $AstNodes$}
		\If{$AstNode$ $is$ Variable Decelerator Node}
		\If{\textbf{"Ndef"} = $AstNode$.name}
		\State append $AstNode$.name \textbf{to} $VarNames$
		\EndIf
		\EndIf
		\If{$AstNode$ $is$ Method Invocation Node $and$ $AstNode$.qualifier $in$ $VarNames$}
		
		\If{$AstNode$.member = \textbf{"writeNdefMessage"}}
		\State append \textbf{$AstNode$.member} $in$ $MethodInovationList$
		
		\If{$AstNode$.member = \textbf{"createApplicationRecord"}}
		\State append \textbf{$AstNode$.member} $in$ $MethodInovationList$
		
		\EndIf
		\EndIf
		\EndIf
		
		\EndFor
		
		\If{$MethodInovationList$ includes \textbf{"createApplicationRecord"} $and$ \textbf{"writeNdefMessage"}}
		\State \textbf{Return} True
		\EndIf
		
		\State \textbf{Return} False
		
	\end{algorithmic} 
\end{algorithm}

%\section{tables in empirical analysis}

%\label{appendix:tables}

%this appendix contains the tables of empirical analysis

\end{appendices}
